# Supplementary material for: NoviCode: Generating Programs from Natural Language Utterances by Novices
Source: arXiv:2407.10626 source file (2024-07-16)
Supplement: Supplementary file 1 [file appendix_error_analysis.tex]

\section{Appendix: Error Analysis Examples}
\label{appendix:error-analysis}

The examples for this error analysis were drawn from the best-performing model (CodeT5+ with 220M parameters using the \texttt{LangCodeRep} setup we proposed).

\subsection{Syntactical Errors}
For the user instruction \textit{"Check the weather for the 4th of July and send a text to Grandpa to invite him over and tell him the weather."}. 
The model generated a linearized output format of the compacted AST form. This is erroneous as the model reached its max token size output and therefore did not correctly close the brackets notations used for the tree representation.

\begin{lstlisting}[style=txt]
[ Module 
    [ date_time = DateTime.resolve_from_text('the 4th of July') ] 
    [ weather_forecasts = Weather.find_weather_forecasts(date_time=date_time) ] 
    [ Responder.respond(response=weather_forecasts) ] [ recipient = Contact.resolve_from_text('Brandpa') ] 
    [ message_content_type = MessageContentType.resolve_from_text('a text') ] 
    [ content = Content.resolve_from_text('invite him over') ] [ Messages.send_message(recipient=recipient, message_content_type=message_content_type, content=content) ] 
    [ product_name = ProductName.resolve_from_text('sandals') ] [ product_attribute = ProductAttribute.resolve_from_text('on sale') ] 
    [ products = Shopping.find_products(product_name=product_name, product_attribute=product_attribute) ] 
    [ Responder.respond(response=products) ]
    [
\end{lstlisting}

\subsection{Logical Errors}
The following example of a logical error exemplifies an incorrect usage of the API where a method (\texttt{Navigation.find\_duration()}) is called with an unexpected argument (\texttt{date\_time} whereas the API call expected a \texttt{departure\_date\_time} argument).

\begin{lstlisting}[style=python]
date_time = DateTime.resolve_from_text('8pm')
duration = Navigation.find_duration(
    destination=destination, 
    date_time=date_time
)
\end{lstlisting}

\subsection{Semantic Errors}
\subsubsection*{Calling the wrong API}
In the following example, the model generates a program code that calls a function in an unrelated domain.

For the user request: "\textit{Set timer to wake me up in 3 hours at 5, 6, 7 AM.}"

The model calls a function from the product API specification while it should have been using the Clock domain function to set a timer. The model generated the following code:

\begin{lstlisting}[style=python]
product_name = ProductName.resolve_from_text('timer')
product_attribute = ProductAttribute.resolve_from_text('set')
location = Location.resolve_from_text('Wake me up in 3 hours')
products = Shopping.find_products(
    product_name=product_name, 
    product_attribute=product_attribute, 
    location=location
)
Responder.respond(response=products)
\end{lstlisting}

\subsubsection*{Irrelevant information in the output}
The model was seen to create outputs with irrelevant information that was not specified in the NL user utterance.

For instance, the original user request was as follows: "\textit{Can you place an order for two turkeys to arrive the 22nd, and remind me about it on the 21st?}"

Yet, the model generated a resultant code that included terms that were never mentioned in the above user request. The code includes phrases like 
\textit{'the a/c is broken or lock the door'}.

\begin{lstlisting}[style=python]
amount = Amount.resolve_from_text('2')
product_name = ProductName.resolve_from_text('tur keys')
shopping_list_name = ShoppingListName.resolve_from_text('arrival')
locations = Location.resolve_many_from_text('the 22nd, I have a meeting at 3pm or close the window')
order = []
for location in locations:
    order += Shopping.order(product_name=product_name, amount=amount, shopping_list_name=shopping_list_name, location=location)
date_time = DateTime.resolve_from_text('the 21st?')
person_reminded = Contact.resolve_from_text('me')
contents = Content.resolve_many_from_text('the a/c is broken or lock the door')
\end{lstlisting}

\subsubsection*{Low recall in arguments capturing}
Correctly recognizing and gathering the essential arguments to fulfill a user's natural language request is key to accurately generating the desired code. Users typically provide details of their intents through straightforward descriptions. However, elements within the same phrase structures (like \textsc{NP}, \textsc{PP}, or \textsc{ADJP}) that should be converted into arguments were sometimes partly overlooked or mistakenly combined into a single data type.

For example, considering the utterance \textit{If the weather is cold tomorrow please remind me to grab my winter jacket}. The model generated output that resulted in the below code (only the relevant section is brought for this example). The user intended to condition the reminder action in the possibility of the weather being cold tomorrow. Yet, the model did not capture the weather attribute \texttt{cold}.

\begin{lstlisting}[style=python]
date_time = DateTime.resolve_from_text('tomorrow')
weather_forecasts = Weather.find_weather_forecasts(date_time=date_time)
\end{lstlisting}

\subsubsection*{Implicit conditions}

\subsubsection*{Implicit and explicit loops}
Loops and iterative actions are inferred explicitly by using noun phrases in conjunction (e.g. \textit{Monday night and Tuesday morning}) or implicitly from the NL instructions by including quantifiers (e.g. \textit{all my friends}) or other semantic notations (e.g. \textit{my chess club}). 
While the model seemed to be successful with recovering the explicit cases and outputting control flow structures of for-loops, it was unable to translate implicit cases to correct for-loops.

\subsubsection*{Variable reusability}
In this example of coreference within a user description, the model does not reuse a predefined variable and re-define an identical variable.

NL User description: \\
\textit{Check there are messages from Jane and reply to her messages with "I am busy!"}

In the generated code, the model defines multiple time the \texttt{recipient} variable, though in the NL command it is declared through a coreference anaphor (\textit{her})
\begin{lstlisting}[style=python]
sender = Contact.resolve_from_text('Jane')
messages = Messages.find_messages(sender=sender)
test_messages = bool(messages)
Responder.respond(response=test_messages)
message_content_type = MessageContentType.resolve_from_text('reply')
recipient = Contact.resolve_from_text('Jane')
content = Content.resolve_from_text('I am busy on Thursday')
Messages.send_message(recipient=recipient, content=content, message_content_type=message_content_type)
\end{lstlisting}

\subsubsection*{Ambiguity in the NL instructions}
For example, in the instruction \textit{"Text John to read it in 10 minutes"}, the time notation \textit{"in 10 minutes"} can be interpreted as the time parameter to the \texttt{send\_message} action or as part of the full content of the message.
