# Supplementary material for: NoviCode: Generating Programs from Natural Language Utterances by Novices
Source: arXiv:2407.10626 source file (2024-07-16)
Supplement: Supplementary file 2 [file appendix_open_ai.tex]

\section{Appendix: In-context Learning Prompts Used in Research}
\label{appendix:in-context-prompt}

This appendix provides detailed information about the specific prompts used in LLMs in our research. Each prompt is listed with its intended purpose and any relevant context or observations made during the study.

\subsection*{Few-shot Learning with Examples}
% \addcontentsline{toc}{subsection}{Few-shot Learning with Examples}

\paragraph{Overview}
We used a few-shot prompt embedded with multiple pairs of input and matching output examples to train and evaluate the LLMs' ability to accurately translate non-technical NL descriptions into corresponding executable code adhering to a specific API.
We used 18 examples of synthesized examples. This number fitted the smallest input context window in our experiment.
The different input-output setups we experimented with are shown in Table~\ref{tab:experiment-setup}.

\paragraph{Prompt 1: Few-shot examples prompt for text-to-code}
\textbf{Purpose:} We tested a text-to-code approach where the input was an NL text description and the desired output was executable program code. Below is the prompt template that illustrates the structure we used in this setup.
\newline
\textbf{Prompt:}
\begin{lstlisting}[style=txt]
[
    {
        "role": "system", 
        "content": "You are a skilled programmer. You will be provided with a text description and your task is to convert it into Python code."
    },
    {
        "role": "user",
        "content": "Below are examples of text descriptions and their corresponding Python code implementations.
        Text: <example text>"
    }, 
    {
        "user": "assistant",
        "content": "Code: <example code>"
    },
    {
        "role": "user",
        "content": Text: <example text>"
    }, 
    {
        "user": "assistant",
        "content": "Code: <example code>"
    },
    ...
    {
        "role": "user",
        "content": "Based on the previous examples, convert the following text to code.
        Text: <text>"
      }
]
\end{lstlisting}

\paragraph{Prompt 3: Few-shot examples prompt for an NL description to a dense AST form}
\textbf{Purpose:} We tested a setup where the input was an NL description and the desired output was our code representation form of a dense AST. Below is the prompt template that illustrates the structure we used in this setup.

\newline
\textbf{Prompt:}
\begin{lstlisting}[style=txt]
[
    {
        "role": "system", 
        "content": "You are a skilled programmer. You will be provided with a variation of a Universal Dependencies (UD) tree and your task is to convert it into Python code."
    },
    {
        "role": "user",
        "content": "Below are examples of variations of Universal Dependencies (UD) trees and their corresponding Python code implementations.
        Text: <example text>"
    }, 
    {
        "user": "assistant",
        "content": "Code: <example code>"
    },
    {
        "role": "user",
        "content": Text: <example text>"
    }, 
    {
        "user": "assistant",
        "content": "Dense AST: <example dense AST>"
    },
    ...
    {
        "role": "user",
        "content": "Based on the previous examples, convert the following text description into Python dense AST form
        Text: <example text>"
      }
]
\end{lstlisting}

\subsection*{API Specifications In-context Prompt}
% \addcontentsline{toc}{subsection}{API Specifications In-context Prompt}

\paragraph{Overview}
We expanded our in-context prompt to encompass the full API specifications, augmenting the few-shot examples with detailed API information. The original prompt structure was maintained, but we added an extra set of user-assistant interactions that clearly outlined the complete API specifications.
\newline
The following is an example of the text-to-code prompt augmented with the API specifications. 
\newline
\textbf{Prompt:}
\begin{lstlisting}[style=txt]
[
    {
        "role": "system", 
        "content": "You are a skilled programmer. You will be provided with a text description and your task is to convert it into Python code."
    },
    {
        "role": "user",
        "content": <Full API specification>
    },
    {
        "role": "assistant",
        "content": "ok"
    }
    {
        "role": "user",
        "content": "Below are examples of text descriptions and their corresponding Python code implementations.
        Text: <example text>"
    }, 
    {
        "user": "assistant",
        "content": "Code: <example code>"
    },
    {
        "role": "user",
        "content": Text: <example text>"
    }, 
    {
        "user": "assistant",
        "content": "Code: <example code>"
    },
    ...
    {
        "role": "user",
        "content": "Based on the API spec and previous examples, convert the following text to code.
        Text: <text>"
      }
]
\end{lstlisting}
