# Supplementary material for: NoviCode: Generating Programs from Natural Language Utterances by Novices
Source: arXiv:2407.10626 source file (2024-07-16)
Supplement: Supplementary file 3 [file appendix_examples.tex]

\subsection{Utterances description} 
\label{appendix:examples}
